# Supplementary material for: Manipulation and control of temporal cavity solitons with trapping potential
Source: arXiv:2406.12848 source file (2024-06-18)
Supplement: Supplementary file 1 [file SM.pdf]

# Supplemental Material – Manipulation and control of temporal cavity solitons with trapping potentials

Nicolas Englebert,[1,2] Corentin Simon,[1] Carlos Mas Arabí,[1,3] François Leo,[1] and Simon-Pierre Gorza[1,*]

[1]*Service OPERA-Photonique, Université libre de Bruxelles (U.L.B.), 50 Avenue F. D. Roosevelt, CP 194/5, B-1050 Brussels, Belgium*

[2]*Department of Electrical Engineering, California Institute of Technology, Pasadena, California 91125, USA*

[3]*Institut Universitari de Matemàtica Pura i Aplicada, Universitat Politècnica de València, 46022 (València), Spain*

**Contents**

A. Modelling - Driven-dissipative Gross-Pitaevskii equation 1
1. Dimensional form 1
2. Normalized form 2
B. Reduced model – Equations of motion 2
1. Dimensional form 2
2. Normalized form 3
C. Cancellation of the Raman-induced self-frequency shift by external potentials: limit of shortest CSs 3
D. Schematic of the experimental set-up 4
E. Bloch oscillations of the Kelly bands 5
F. Internal versus external phase modulation 6
G. Supplementary Figure 7

**References** 7

## A. Modelling - Driven-dissipative Gross-Pitaevskii equation

### 1. Dimensional form

The dynamics of Kerr cavity solitons (CSs) in trapping potentials $\overline{V}$ can be described by a Lugiato-Lefever equation (LLE) [1, 2], generalized to account for the intracavity phase modulation, $\phi_{\text{int}} = \overline{V}$, [3] and the stimulated Raman scattering (SRS) [4, 5]. Such generalization corresponds to a driven-dissipative Gross-Pitaevskii equation, which reads:

$$t_{\text{R}}\frac{\partial E}{\partial t} = \left(-\frac{\Lambda_e}{2} - i\left[\delta_0 - \overline{V}(\tau)\right] + \left[t_R \bar{d}\frac{\partial}{\partial \tau} - i\frac{\beta_2 L_c}{2}\frac{\partial^2}{\partial \tau^2}\right] + i\gamma L_c\left[E^2 - \overline{\tau_R}\frac{\partial |E|^2}{\partial \tau}\right]\right)E + \sqrt{\theta P_{\text{in}}} \tag{S1}$$

where $t_{\text{R}} = \text{FSR}^{-1}$ is defined as the inverse of the cavity free spectral range (FSR) and corresponds to the cavity roundtrip time at the driving wavelength. $t$ is the (slow) time describing the evolution of the electric field envelope $E(t,\tau)$ with $\tau$, a (fast) time variable defined in a co-moving reference frame in which the potential $\overline{V}(\tau)$ is stationary with time $t$. $\Lambda_e = -\ln(T\times G)$ denotes the effective cavity loss that takes into account the "cold cavity" transmission ($T$) and the intracavity gain of the optical amplifier (amplification factor $G$) [6]. The phase detuning between the driving field and the closest cavity resonance is $\delta_0 = 2\pi m - \beta L_c$, with $L_c$, the cavity length, $\beta$, the propagation constant, and $m$, an integer. $\beta_2$ and $\gamma$ are, respectively, the group-velocity dispersion and the nonlinear Kerr coefficient of the resonator. $\overline{\tau_R}$ is the Raman time constant. $\theta$ and $P_{\text{in}}$ are the input coupler ratio and coherent driving power, respectively. Finally, $\bar{d}$ is the drift coefficient of a wave at the driving frequency in the reference frame co-moving with the potential. For an intracavity phase modulation of the form $J_{\text{RF}}\cos(\omega_{\text{RF}}t)$, we thus have $\overline{V} = J_{\text{RF}}\cos(\omega_n\tau)$ and $\bar{d} = \Delta\omega/\omega_n$, where $\Delta\omega = \omega_n - \omega_{\text{RF}}$ is the frequency difference between the n$^{th}$ harmonic of the cavity FSR ($\omega_n = n\times 2\pi\times\text{FSR}$) and the modulation frequency.

---

*Electronic address: simon.pierre.gorza@ulb.be

### 2. Normalized form

It is convenient to introduce dimensionless parameters to carry out theoretical analyses and draw general conclusions. Choosing the usual LLE normalization with $\tau_c = \sqrt{-\beta_2 L_c/\Lambda_e}$ and $\alpha_e = \Lambda_e/2$ [2]:

$$t \to \frac{\alpha_e t}{t_R}, \qquad \tau \to \frac{\tau}{\tau_c}, \qquad A = E\sqrt{\frac{\gamma L_c}{\alpha_e}}, \qquad S = \sqrt{\frac{\gamma L_c \theta_{\rm in} P_{\rm in}}{\alpha_e^3}}, \tag{S2}$$
$$\Delta = \frac{\delta_0}{\alpha_e}, \qquad V = \frac{\overline{V}}{\alpha_e}, \qquad d = \bar{d}\frac{t_R}{\tau_c \alpha_e}, \qquad \tau_R = \frac{\overline{\tau_R}}{\tau_c},$$

Eq. (S1) becomes:

$$\frac{\partial A(t,\tau)}{\partial t} = S + \left( -1 - i\Big[\Delta - V(\tau)\Big] + i\left[|A|^2 - \tau_R \frac{\partial |A|^2}{\partial \tau}\right] + \left[d\frac{\partial}{\partial \tau} + i\frac{\partial^2}{\partial \tau^2}\right]\right)A, \tag{S3}$$

which corresponds to Eq. (1) of the main manuscript when $\tau_R = 0$.

## B. Reduced model – Equations of motion

### 1. Dimensional form

There are no known closed-form analytical expressions that would describe CS solutions of the mean-field equation (S1), with or without the SRS term. However, equations of motion can be found by using a perturbative Lagrangian approach [7]. Starting with the soliton ansatz [5, 7]:

$$E_s(t,\tau) = \overline{B}\,\mathrm{sech}\left(\frac{\overline{B}(\tau - \tau_s)}{\sqrt{-\beta_2/\gamma}}\right) \mathrm{e}^{-i\overline{\Omega}(\tau-\tau_s)}\mathrm{e}^{i\overline{\phi}} \tag{S4}$$

where $\overline{\Omega}$ corresponds to the soliton central frequency, $\overline{B}$ is the soliton amplitude (with units of $\mathrm{W}^{1/2}$), $\tau_s$ is the soliton position along the fast-time, and $\overline{\phi}$ is the cavity soliton phase. Following the procedure described in [5, 7, 8], one can find the equations of motion for each of the CS (dimensional) parameters:

$$\begin{aligned}
t_R\frac{d\overline{\Omega}}{dt} &= -\frac{\overline{\Omega}}{\overline{B}}t_R\frac{d\overline{B}}{dt} - 2\alpha_e\overline{\Omega} - \frac{d\overline{V}(\tau_s)}{d\tau_s} + \frac{8\overline{\tau_R}\gamma^2 L_c}{15\beta_2}\overline{B}^4,\\
t_R\frac{d\overline{B}}{dt} &= -2\alpha_e\overline{B} + \pi\sqrt{\theta P_{\rm in}}\cos(\overline{\phi})\,\mathrm{sech}\left(\sqrt{\frac{-\beta_2}{\gamma}}\frac{\overline{\Omega}\pi}{2\overline{B}}\right),\\
t_R\frac{d\tau_s}{dt} &= \beta_2 L_c\overline{\Omega} - t_R\bar{d} + \frac{\pi^2}{2\overline{B}^2}\sqrt{\frac{-\beta_2}{\gamma}\theta P_{\rm in}}\sin(\overline{\phi})\,\mathrm{sech}\left(\sqrt{\frac{-\beta_2}{\gamma}}\frac{\overline{\Omega}\pi}{2\overline{B}}\right)\tanh\left(\sqrt{\frac{-\beta_2}{\gamma}}\frac{\overline{\Omega}\pi}{2\overline{B}}\right),\\
t_R\frac{d\overline{\phi}}{dt} &= \frac{\gamma L_c\overline{B}^2}{2} + \frac{\beta_2 L_c}{2}\overline{\Omega}^2 - [\delta_0 - \overline{V}(\tau_s)] - t_R\overline{\Omega}\left[\frac{d\tau_s}{dt} + \bar{d}\right]\\
&\quad + \frac{\pi^2}{2\overline{B}^2}\overline{\Omega}\sqrt{\frac{-\beta_2}{\gamma}\theta P_{\rm in}}\sin(\overline{\phi})\,\mathrm{sech}\left(\sqrt{\frac{-\beta_2}{\gamma}}\frac{\overline{\Omega}\pi}{2\overline{B}}\right)\tanh\left(\sqrt{\frac{-\beta_2}{\gamma}}\frac{\overline{\Omega}\pi}{2\overline{B}}\right),
\end{aligned} \tag{S5}$$

### 2. Normalized form

Applying the normalization Eq. (S2) to the system of equations (S5) and neglecting the terms proportional to $B^{-2}$ yield Eqs. (2)-(5) of the main manuscript (for $\tau_R = 0$):

$$\begin{aligned}
\frac{d\Omega}{dt} &= -\frac{\Omega}{B}\frac{dB}{dt} - 2\Omega - \frac{dV(\tau_s)}{d\tau_s} - \frac{4\tau_R}{15}B^4, \\
\frac{dB}{dt} &= -2B + \pi S\cos(\phi)\,\mathrm{sech}\left(\frac{\Omega\pi}{\sqrt{2}B}\right), \\
\frac{d\phi}{dt} &= \frac{B^2}{2} - \Omega^2 - [\Delta - V(\tau_s)] - \left(\frac{d\tau_s}{dt} + d\right)\Omega, \\
\frac{d\tau_s}{dt} &= -2\Omega - d.
\end{aligned} \tag{S6}$$

## C. Cancellation of the Raman-induced self-frequency shift by external potentials: limit of shortest CSs

From the motion equations, we can find the conditions under which a potential completely cancels the Raman-induced frequency shift of cavity solitons. To do so, we look at the stationary solutions at $\Omega = 0$ (we note that red- and blue-shifted CSs still exist in the presence of SRS, but we here restrict ourselves to unshifted solutions). The stationary solution of S6 reads:

$$\begin{aligned}
&\Omega = d = 0, \\
&\cos(\phi) = \frac{2B}{\pi S}, \\
&\frac{B^2}{2} = \Delta - V(\tau^*), \\
&\mathcal{D}(\tau^*) = -\frac{4\tau_R}{15}B^4,
\end{aligned} \tag{S7}$$

where $\tau^*$ is the position of the CS in the fast time and $\mathcal{D}(\tau^*) = \frac{dV(\tau)}{d\tau}|_{\tau^*}$ is the local potential gradient.

First, the motion equation for the CS amplitude gives $\cos(\phi) = \dfrac{2B}{\pi S} < 1$, which corresponds to the depletion limit. It implicitly accounts for the local detuning $\Delta^* = \Delta - V(\tau^*)$ through the soliton amplitude $B$. A second existence condition arises from the combination of the two last equations:

$$\Delta = \frac{B^2}{2} + V\left[\mathcal{D}^{-1}\left(-\frac{4\tau_R}{15}B^4\right)\right], \tag{S8}$$

where $\mathcal{D}^{-1}$ is the reciprocal of the potential gradient. We now focus on trapping by parabolic potentials of the form $V(\tau) = -a\tau^2/2 < 0$, for which there is no slope limit and an explicit analytical solution can be found. We note that we do not consider any offset on the potential since this term simply shifts the detuning $[\Delta \to \Delta - V(0)]$. We thus have $V\left[\mathcal{D}^{-1}(x)\right] = -\dfrac{x^2}{2a}$, which yields:

$$\Delta = \frac{B^2}{2} - \frac{1}{2a}\left(\frac{4\tau_R}{15}\right)^2 B^8 = \frac{B^2}{2} - \frac{1}{8}\frac{B^8}{B_{\mathrm{max}}^6}, \tag{S9}$$

where we have introduced $B_{\mathrm{max}} = (225a/64\tau_R^2)^{1/6}$ for convenience (see below). The right-hand side of this later equation shows that there is a maximum possible value for $\Delta$ (see also Fig.1). It is found by looking at the soliton amplitude such that $\partial\Delta/\partial B = 0$, which occurs at $B = B_{\mathrm{max}}$ and $\Delta = \Delta_{\mathrm{max}} = (3/8)B_{\mathrm{max}}^2$. This gives the maximum peak power $B_{\mathrm{max}}^2$ of stable CSs for which the interaction with the intracavity phase modulation can cancel the SRS. We note that this limit is independent of the driving amplitude $S$. In conclusion, there are two limitations:

$$B < B_{\mathrm{max}} \quad \text{and} \quad B < \frac{\pi S}{2}. \tag{S10}$$

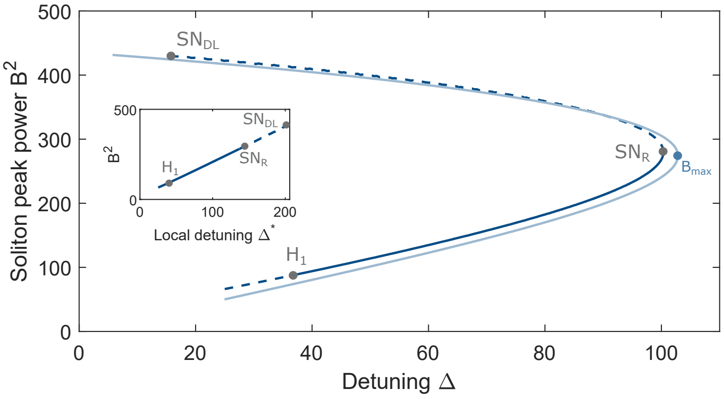


**Fig. S1.** Peak power of the cavity solitons as a function of the detuning $\Delta$ with a trapping parabolic potential and when considering the Raman self-frequency shift. The parameters are $\tau_R = 1.5 \times 10^{-3}$ ($\overline{\tau_R} = 3\,\text{fs}$[4], $\tau_c = 2\,\text{ps}$), $S = 30$, and $a = 13.2$ [parabolic approximation of a cosine modulation at frequency $\mathcal{W} = 0.25$ ($\nu_{\text{RF}} = 20\,\text{GHz}$) and $J = 209$]. The dark blue line shows results from the numerical continuations of solutions of the mean-filed model, where unstable solutions are indicated in dashed lines. $\text{H}_1$, Hopf bifurcation that stabilizes the solution. The two saddle-node bifurcations, $\text{SN}_\text{R}$ and $\text{SN}_\text{DL}$, correspond to the conditions $B = B_{\text{max}}$ and $B = \pi S/2$, respectively. For detunings $\Delta$ below $\text{SN}_\text{R}$, there are two different soliton solutions, with different positions $\tau^*$ and local detuning $\Delta^*$ (see also inset), but only one is stable. Equation (S9) is plotted in light blue. We note a very good agreement between the two models regarding the peak power (and thus the soliton duration) at the saddle-node $\text{SN}_\text{R}$.

Looking at the SRS limitation and applying the denormalization $a \to \bar{a}\tau_c^2/\alpha_e$ [see also Eq. (S2)], the corresponding minimum CS duration in dimensional units reads:

$$\text{FWHM}_{\text{min}} = 4\sqrt{2}\ln\left(1+\sqrt{2}\right)\sqrt[3]{\frac{1}{15}}\left(\frac{\alpha_e\tau_c^2\overline{\tau_R}^2}{\bar{a}}\right)^{1/6} \approx 2.02\left(\frac{\alpha_e\tau_c^2\overline{\tau_R}^2}{\bar{a}}\right)^{1/6}. \tag{S11}$$

Considering the parabolic approximation of a cosine potential of the form $\overline{V} = J_{\text{RF}}\cos(\omega_{\text{RF}}\tau)$, we have $\bar{a} = J_{\text{RF}}\omega_{\text{RF}}^2$. It follows Eq.(9) of the main manuscript. This limit is in excellent agreement with the results of the numerical continuations (Figure S1) of the solutions of the mean-field model. We finally note that exact cosine potentials can also be solved. In this case, finding the maximum CS amplitude for which $\partial\Delta/\partial B = 0$ requires computing the unique positive root of a third-order polynomial.

### D. Schematic of the experimental set-up

Figure S4 depicts the full experimental setup used to investigate the dynamics of cavity solitons in trapping potentials. It consists of an active fiber ring resonator [6] of length $L_c = 64\,\text{m}$ (free spectral range of 3.12 MHz, $\tau_c$=7 ps). Specifically, it is made of 63 m of standard telecommunication single-mode fibre (SMF-28, $\gamma = 1.3\,\text{W}^{-1}\text{km}^{-1}$, $\beta_2 = -2.3 \times 10^{-26}\,\text{s}^2\text{m}^{-1}$ ) spliced to a 75 cm-long segment of erbium-doped fibre (EDF, Liekki® ER16-8/125). The aim of the doped fiber is to partially compensate for the high cavity roundtrip loss ($T = -2.8\,\text{dB}$ when the EDF is removed, corresponding to an intrinsic finesse $\mathcal{F} = 9.7$). The length of the amplifying section has been carefully adjusted following the method described in ref. [6]. The EDF is pumped by a 1480 nm laser through a wavelength division multiplexer, with a power $P_p^{\text{in}} = 2\,\text{W}$. The unabsorbed pump power $P_p^{\text{out}}$ after the EDF is rejected by a second WDM. In addition, to individually address a soliton by means of a single writing pulse [9, 10], the cavity includes a 1535/1550 WDM. The writing pulses come from a 1535 nm mode-locked laser and are gated using an acousto-optic modulator (not shown). The three WDMs combined spectral transmission prevents lasing at shorter wavelengths [10]. With intracavity amplification, the effective loss at small signal is $\Lambda_e = 3\%$ (effective finesse $\mathcal{F}_e = 209$), while the saturation power (neglected in the mean-field simulations) is estimated to 250 mW. The resonator includes an electro-optic phase modulator to generate the (real) potential. The EOM is driven by a harmonic RF signal whose amplitude ($J_{\text{RF}}$) and frequency ($\nu_{\text{RF}}$) can be freely chosen. $J_{\text{RF}}$ is experimentally limited to 1 rad at the modulation frequency ($\approx$ 12 GHz). In addition, an intracavity polarization controller limits the EOM polarization-dependent insertion loss (not shown). The optical cavity is coherently driven with a sub-100-Hz continuous wave laser, centered on 1550.12 nm. It is amplified by a commercial erbium-doped fiber amplifier (EDFA) before being injected into the cavity through

the 90/10 input coupler. The driving beam polarization is adjusted at the cavity input with a polarization controller to excite one eigen polarization mode of the cavity. Part of the intracavity power is extracted at the output coupler (99/1) to perform spectral measurements of the intracavity field. We note that the intracavity phase modulation prevents the build-up of stimulated Brillouin scattering. Therefore, there is no need for an optical isolator, even if the cavity is pumped by a highly coherent CW laser. This enables sending a co-polarized counter-propagating CW control signal to stabilize the cavity detuning. Its polarization is identical to the driving beam to avoid large insertion loss in the EOM. The cavity detuning is actively stabilized by using a proportional-integral-derivative (PID) controller fed by the signal generated by the output control beam on a photodiode (200 kHz bandwidth). The cavity detuning is tuned by slightly shifting the frequency of the control signal with a frequency shifter (FS).

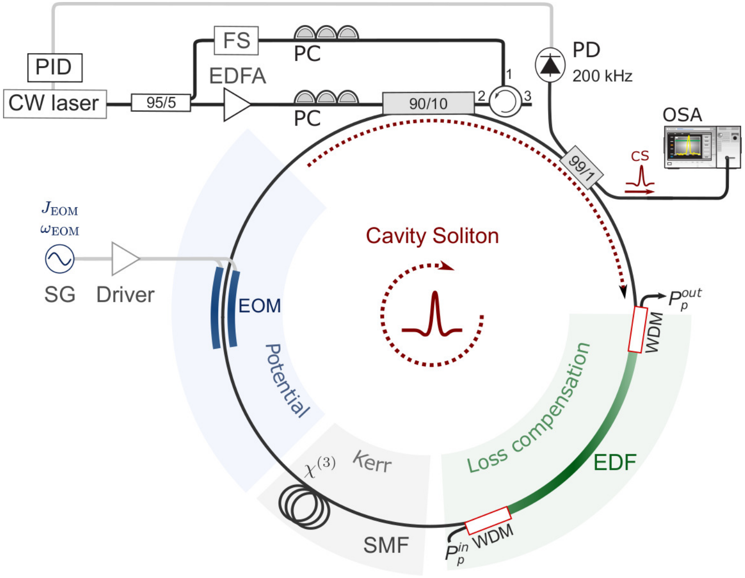


**Fig. S2.** Schematic of the coherently-driven fiber ring active Kerr cavity with intracavity phase modulation. CW laser, continuous-wave laser, FS, frequency shifter, EDFA, optical amplifier, PC, polarization controller, EDF, erbium-doped fiber, SMF, standard single-mode fiber, EOM, electro-optic modulator, WDM, wavelength division multiplexer, SG, radio-frequency (RF) signal generator, Driver, RF amplifier, PD, photodiode, OSA, optical spectrum analyzer, PID: stabilization control electronics.

### E. Bloch oscillations of the Kelly bands

The electro-optic phase modulator included in the fiber loop introduces a coupling between the modes of the resonator with a strength given by $J = J_{\rm RF}/(2t_R)$ for a modulation $J_{\rm RF}\cos(2\pi\nu_{\rm RF}t)$, where $\nu_{\rm RF}$ is a frequency close to an integer multiple ($n$) of the FSR. These coupled sites form a synthetic 1D lattice along the frequency axis [8]. By detuning the modulation from a resonant frequency ($\nu_{\rm RF} = n \times {\rm FSR} + \Delta f$), an effective force along the frequency axis is implemented. This force, which is responsible for the Bloch oscillations (BOs) in the synthetic frequency lattice, is given by:

$$F = đ = \frac{n \times {\rm FSR} - \nu_{\rm RF}}{n \times {\rm FSR}}. \tag{S12}$$

Assuming that the modulation is resonant at the driving frequency $\omega_0$ ($\nu_{\rm RF} = n_0 \times {\rm FSR}|_{\omega_0}$), this modulation becomes detuned from resonance at $\omega$ because of chromatic dispersion. We thus have $\Delta f = n_0({\rm FSR}|_{\omega_0} - {\rm FSR}|_{\omega}) \approx \frac{\beta_2}{\beta_1} n_0 {\rm FSR}|_{\omega_0} \times (\omega - \omega_0)$. The effective force thus reads:

$$F \approx \frac{\Delta f}{\nu_{\rm RF}} = \frac{\beta_2}{\beta_1}\Delta\omega, \tag{S13}$$

where $\Delta\omega = \omega - \omega_0$.

BOs are characterized by an oscillation amplitude $A_{\rm BO} = 2J/F$. This amplitude thus reads:

$$A_{\rm BO}|_{\omega} = \frac{J_{\rm RF}\beta_1}{t_R\beta_2}\frac{1}{\Delta\omega} = \frac{J_{\rm RF}}{L_c\beta_2}\frac{1}{\Delta\omega}, \tag{S14}$$

with $t_R = \beta_1 L_c$.

The amplitude of the BOs as a function of the inverse of the frequency shift from the driving is shown in figure 3. The circles denote the data measured from the numerical simulation of the dynamics of CS with a periodic potential, which is reported in Fig.7 of the main manuscript. These results are in excellent agreement with the theoretical model Eq. (S14), confirming that the oscillations of the Kelly bands can be interpreted as Bloch oscillations.

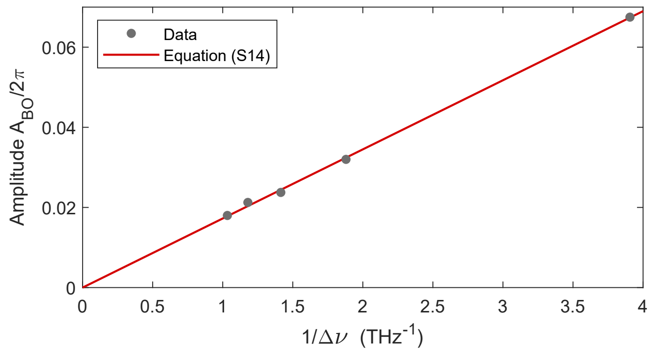


**Fig. S3.** Amplitude of the spectral oscillations of the Kelly sidebands as a function of the inverse of their frequency shift from the driving ($\Delta\nu = \Delta\omega/2\pi$). The circles are the amplitudes extracted from the numerical simulation shown in Fig.7 of the main manuscript. The parameters are $\beta_2 = -2.3 \times 10^{-26}\,\mathrm{s^2m^{-1}}$, $L_c = 64\,\mathrm{m}$. The red line shows the theoretical relation Eq.S14.

## F. Internal versus external phase modulation

Studies of the motion dynamics of cavity solitons in presence of a modulated driving field, either in phase or in amplitude, have revealed that cavity solitons can be manipulated and trapped by the modulations [11–14]. For instance, such trapping as been used to control and stabilize the soliton repetition rate [15], which is interesting for applications. Real potentials, as considered in this work, correspond to phase modulations of the intracavity field. Of particular interest for comparison are, therefore, external purely phase-modulated driving fields.

For an *external* phase modulation, the CS drift velocity in normalized variables reads [14]:

$$v_{\text{ext}} = \frac{d\tau_s}{dt} = 2\phi'_{\text{ext}} - d, \tag{S15}$$

where ' stands for the first derivative with respect to the slow time $\tau$. The corresponding dimensional expression of the drift velocity is:

$$\overline{v}_{\text{ext}} = \frac{L_c}{t_R}|\beta_2|\frac{d\phi_{\text{ext}}}{d\tau}|_{\tau_s} - \bar{d}. \tag{S16}$$

This can be compared with Eq. (5) of the main manuscripts for *internal* phase modulations:

$$v_{\text{int}} = -2\Omega - d, \tag{S17}$$

with $\Omega$ the normalized frequency shift of the CS. Hence, this gives for $\overline{V} = \phi_{\text{int}}$:

$$\overline{v}_{\text{int}} = -\frac{1}{\Lambda_e}\frac{L_c}{t_R}|\beta_2|\frac{d\phi_{\text{int}}}{d\tau}|_{\tau_s} - \bar{d}. \tag{S18}$$

We can see that the equations (S16) and (S18) are identical, providing that

$$\phi_{\text{int}} = \Lambda_e \phi_{\text{ext}}. \tag{S19}$$

This result shows that a phase modulation amplitude $1/\Lambda_e$ times smaller is required for internally modulated resonators to achieve the same effect as with external modulation of the driving beam. The locking range, and hence the maximum frequency shift of the CS or the tuning range of the soliton repetition rate, is thus enhanced by the same factor, which can also be written $\mathcal{F}/2\pi$ or $Q\nu_0/(2\pi \times \text{FSR})$, with $Q$ the resonator $Q$-factor and $\nu_0$ the soliton carrier frequency.

This emphasizes the importance of the loss in the dynamics of CSs in internally modulated resonators as well as the interest of internal modulations for applications.

## G. Supplementary Figure

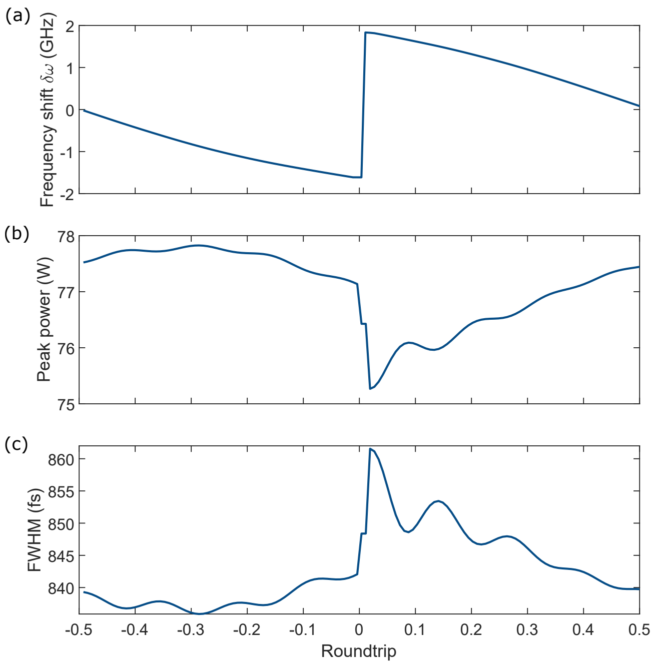


**Fig. S4. Soliton single-roundtrip dynamic.** Evolution of (**a**) the soliton frequency shift, (**b**) peak power, and (**c**) temporal full width at half maximum (FWHM) over one roundtrip. The simulation corresponds to a lumped element model of the system using the following parameters: $L = 64\,\text{m}$, $\gamma = 1.3 \times 10^{-3}\,\text{W}^{-1}.\text{m}^{-1}$, $\beta_2 = -23 \times 10^{-27}\,\text{s}^2.\text{m}^{-1}$, $\delta_0 = 4.1\,\text{rad}$, $P_{\text{in}} = 250\,\text{mW}$, $\theta_{\text{in}} = 0.1$, $J_{\text{RF}} = 1\,\text{rad}$, $\omega_{\text{RF}} = 2\pi \times 11.8\,\text{rad.GHz}$, $\bar{d} = 0$, $\overline{\tau_R} = 3\,\text{fs}$.

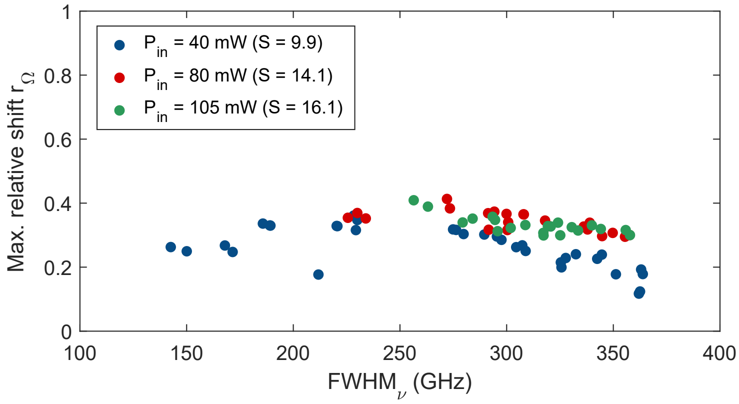


**Fig. S5.** Maximum relative shift $r_\Omega = \Omega/(2\pi \times \text{FWHM}_\nu)$ as a function of the soliton spectral full width at half maximum ($\text{FWHM}_\nu$) for different driving power $P_{in}$ at a fixed modulation amplitude of $J = 66.67$.

[1] L. A. Lugiato and R. Lefever. Spatial Dissipative Structures in Passive Optical Systems. *Physical Review Letters*, 58(21):2209–2211, May 1987.
[2] M. Haelterman, S. Trillo, and S. Wabnitz. Dissipative modulation instability in a nonlinear dispersive ring cavity. *Optics Communications*, 91(5):401–407, August 1992.

[3] Aleksandr K. Tusnin, Alexey M. Tikan, and Tobias J. Kippenberg. Nonlinear states and dynamics in a synthetic frequency dimension. *Physical Review A*, 102(2):023518, August 2020.
[4] A.K. Atieh, P. Myslinski, J. Chrostowski, and P. Galko. Measuring the Raman time constant (T/sub R/) for soliton pulses in standard single-mode fiber. *Journal of Lightwave Technology*, 17(2):216–221, February 1999.
[5] Xu Yi, Qi-Fan Yang, Ki Youl Yang, and Kerry Vahala. Theory and measurement of the soliton self-frequency shift and efficiency in optical microcavities. *Optics Letters*, 41(15):3419–3422, August 2016.
[6] Nicolas Englebert, Carlos Mas Arabí, Pedro Parra-Rivas, Simon-Pierre Gorza, and François Leo. Temporal solitons in a coherently driven active resonator. *Nature Photonics*, pages 1–6, May 2021.
[7] Andrey B. Matsko and Lute Maleki. On timing jitter of mode locked Kerr frequency combs. *Optics Express*, 21(23):28862–28876, November 2013.
[8] Nicolas Englebert, Nathan Goldman, Miro Erkintalo, Nader Mostaan, Simon-Pierre Gorza, François Leo, and Julien Fatome. Bloch oscillations of coherently driven dissipative solitons in a synthetic dimension. *Nature Physics*, 19(7):1014–1021, July 2023.
[9] François Leo, Stéphane Coen, Pascal Kockaert, Simon-Pierre Gorza, Philippe Emplit, and Marc Haelterman. Temporal cavity solitons in one-dimensional Kerr media as bits in an all-optical buffer. *Nature Photonics*, 4(7):471–476, July 2010.
[10] Nicolas Englebert, Carlos Mas Arabí, Simon-Pierre Gorza, and François Leo. High peak-to-background-ratio solitons in a coherently driven active fiber cavity. *APL Photonics*, 8(12):120802, December 2023.
[11] Jae K. Jang, Miro Erkintalo, Stéphane Coen, and Stuart G. Murdoch. Temporal tweezing of light through the trapping and manipulation of temporal cavity solitons. *Nature Communications*, 6(1):7370, June 2015.
[12] Jae K. Jang, Miro Erkintalo, Jochen Schröder, Benjamin J. Eggleton, Stuart G. Murdoch, and Stéphane Coen. All-optical buffer based on temporal cavity solitons operating at 10 Gb/s. *Optics Letters*, 41(19):4526–4529, October 2016.
[13] Yadong Wang, Bruno Garbin, François Leo, Stéphane Coen, Miro Erkintalo, and Stuart G. Murdoch. Addressing temporal Kerr cavity solitons with a single pulse of intensity modulation. *Optics Letters*, 43(13):3192–3195, July 2018.
[14] Miro Erkintalo, Stuart G. Murdoch, and Stéphane Coen. Phase and intensity control of dissipative Kerr cavity solitons. *Journal of the Royal Society of New Zealand*, 0(0):1–19, March 2021.
[15] Daniel C. Cole, Jordan R. Stone, Miro Erkintalo, Ki Youl Yang, Xu Yi, Kerry J. Vahala, and Scott B. Papp. Kerr-microresonator solitons from a chirped background. *Optica*, 5(10):1304–1310, October 2018.
